# Supplementary material for: Action-Value Calibration via Continuation Sharing for Long-Horizon Agentic Reinforcement Learning
Source: arXiv:2610.37195 source file (2026-11-27)
Supplement: Supplementary file 1 [file appendix.tex]

\section{Benchmark Details}
\label{app:benchmarks}
\subsection{WebShop}
WebShop~\citep{yao2022webshop} is a simulated shopping environment in which agents purchase products that satisfy natural-language requests. Following the WebShop setting of GraphGPO~\citep{cheng2026graphgpo}, we adopt the text-rich interface, which presents page content and identifies interactive elements. We conduct experiments in the 1,000-product environment with programmatically generated goals. Goals with indices 0--499 form the evaluation pool, and the remaining goals form the training pool. Each episode allows up to 15 environment interactions. The environment assigns the purchased product a match score in $[0,1]$ based on its type, attributes, selected options, and price relative to the request. We report \textit{task score} as the mean match score multiplied by 100 and \textit{success rate} as the percentage of episodes with a match score of 1. Task score captures partial satisfaction of the requirements, whereas success rate measures complete task fulfillment.

\subsection{ALFWorld}
ALFWorld~\citep{shridhar2021alfworld} provides household tasks that require agents to follow natural-language instructions through sequential interactions. The six task categories are \textit{Pick}, \textit{Clean}, \textit{Cool}, \textit{Look}, \textit{Heat}, and \textit{Pick2}. These tasks involve locating objects and completing prerequisite actions in the appropriate order. Training tasks are drawn from the 3,553 games in the training split, and evaluation tasks are drawn from the 140 games in the held-out seen split. Each episode allows up to 50 environment interactions. An episode is successful when all task goal conditions are satisfied within this limit. We report success rates for each task category and an overall success rate (\textit{All}) computed across all evaluated episodes.

\section{Implementation Details}
\label{app:implementation}

\paragraph{Training configuration.}
We implement ConCal in verl-agent~\citep{feng2025gigpo} with FSDP for policy training and vLLM for rollout generation. We retain the actor-loss reduction used in GiGPO. We fully fine-tune Qwen2.5-1.5B-Instruct and Qwen2.5-VL-3B-Instruct on two NVIDIA H100 GPUs per run, and Qwen2.5-7B-Instruct on four. Each GPU has 80\,GB of memory. We adopt AdamW with a constant learning rate, no warmup, and $(\beta_1,\beta_2)=(0.9,0.999)$. For ALFWorld and WebShop, we assign a terminal task reward of 10 for successful completion and 0 otherwise, with an additional penalty for invalid actions. Following GiGPO, invalid-action penalties are applied separately from continuation calibration, before step-advantage normalization. We compute step advantages with batch-wise normalization as detailed in Appendix~\ref{app:step_normalization}, while episode-level advantages follow GiGPO. \tablename~\ref{tab:hyperparameters} summarizes the training and evaluation settings.

\begin{table}[t]
\centering
\small
\renewcommand{\arraystretch}{1.08}
\setlength{\tabcolsep}{3pt}
\resizebox{\columnwidth}{!}{%
\begin{tabular}{@{}lccc@{}}
\toprule
Hyperparameter & ALFWorld & WebShop & Sokoban \\
\midrule
Training updates & 150 & 150 & 150 \\
Tasks per update & 16 & 16 & 32 \\
Trajectories per task & 8 & 8 & 8 \\
Retained interaction steps & 2 & 2 & 2 \\
Maximum environment steps & 50 & 15 & 15 \\
Maximum input tokens & 2,048 & 5,120 & 1,024 \\
Maximum response tokens & 512 & 512 & 512 \\
\midrule
Actor learning rate & $10^{-6}$ & $10^{-6}$ & $10^{-6}$ \\
Weight decay & $0.01$ & $0.01$ & $0.01$ \\
PPO mini-batch size & 256 & 64 & 64 \\
PPO epochs per update & 1 & 1 & 1 \\
PPO clipping threshold & $0.2$ & $0.2$ & $0.2$ \\
Gradient clipping norm & $1.0$ & $1.0$ & $1.0$ \\
KL coefficient & $0.01$ & $0.01$ & $0.01$ \\
Invalid-action penalty & $-0.1$ & $-0.1$ & $-0.1$ \\
Discount factor $\gamma$ & $0.95$ & $0.95$ & $0.95$ \\
Local advantage weight $\beta$ & $1.0$ & $1.0$ & $1.0$ \\
\midrule
Training temperature & $1.0$ & $1.0$ & $1.0$ \\
Evaluation temperature & $0.4$ & $0.4$ & $0.4$ \\
Top-$p$ & $1.0$ & $1.0$ & $1.0$ \\
Evaluation episodes & 128 & 128 & 128 \\
Evaluation interval (updates) & 5 & 5 & 5 \\
\bottomrule
\end{tabular}%
}
\caption{Training and evaluation hyperparameters for ConCal.}
\label{tab:hyperparameters}
\end{table}

\noindent\textbf{Evaluation protocol.}
Unless otherwise stated, we follow the evaluation protocol of GraphGPO~\citep{cheng2026graphgpo}. Checkpoints are saved and evaluated every five updates. For each run, we select the checkpoint with the highest validation success rate from the final three saved checkpoints. Main results report the mean and sample standard deviation across three independent training runs.



\section{Algorithm Details}
\label{app:algorithm}
Algorithm~\ref{alg:concal} summarizes the action-value estimation and policy optimization procedures of ConCal. Normalization details are provided in Appendix~\ref{app:step_normalization}.

\begin{algorithm*}[t]
\caption{ConCal}
\label{alg:concal}
\small
\begin{algorithmic}[1]
\Require Rollout batch $\mathcal B$, original episode advantages $\{A^{E,(i)}\}$, current policy $\pi_\theta$, frozen policies $\pi_{\mathrm{old}}$ and $\pi_{\mathrm{ref}}$
\Require Interaction limit $H$ with $T_i\le H$, discount $\gamma$, local advantage weight $\beta$
\Require PPO clipping threshold $\epsilon$, KL coefficient $\lambda_{\mathrm{KL}}$
\Ensure Updated policy $\pi_\theta$

\State Define visits $\mathcal I=\{(i,t)\mid\tau_i\in\mathcal B,\ 0\le t<T_i\}$, with $x_i$ denoting the task of $\tau_i$. Adopt $\mathrm{START}$ as the marker for $s_{-1}^{(i)}$ and $a_{-1}^{(i)}$
\State Construct $z_t^{(i)}=(x_i,s_{t-1}^{(i)},a_{t-1}^{(i)},s_t^{(i)})$ and sharing pools $\mathcal C(z)=\{(i,t)\in\mathcal I\mid z_t^{(i)}=z\}$
\State For each pool, set $n_z\gets\bigl|\{i:\exists t,\ (i,t)\in\mathcal C(z)\}\bigr|$ and $\alpha_z\gets n_z/(n_z+1)$
\State Initialize $\widehat V_0(s_t^{(i)})\gets0$ for all visits and $\widehat V_b(s_{T_i}^{(i)})\gets0$ for all $i$ and $b=0,\ldots,H$

\For{$b=1,\ldots,H$}
    \State $Y_{t,b}^{(i)}\gets r_t^{(i)}+\gamma\widehat V_{b-1}(s_{t+1}^{(i)})$ for all $(i,t)\in\mathcal I$
    \State $\mu_b(z)\gets|\mathcal C(z)|^{-1}\sum_{(j,u)\in\mathcal C(z)}Y_{u,b}^{(j)}$ for every sharing pool
    \State $\widehat V_b(s_t^{(i)})\gets(1-\alpha_z)Y_{t,b}^{(i)}+\alpha_z\mu_b(z)$ for all $(i,t)\in\mathcal I$, with $z=z_t^{(i)}$
\EndFor

\State $\widetilde Q_t^{(i)}\gets r_t^{(i)}+\gamma\widehat V_{H-t-1}(s_{t+1}^{(i)})$ for all $(i,t)\in\mathcal I$
\State Form state groups $\mathcal S_t^{(i)}=\{(j,u)\in\mathcal I\mid x_j=x_i,\ s_u^{(j)}=s_t^{(i)}\}$ and compute their means $\overline{\widetilde Q}_{\mathcal S}$
\State $\Delta_t^{(i)}\gets\widetilde Q_t^{(i)}-\overline{\widetilde Q}_{\mathcal S_t^{(i)}}$ for all visits
\State Compute reference step advantages $A^{S,\mathrm{ref}}$ by applying the reference normalization to the calibrated values within each state group
\State Initialize $\widetilde d_{\mathcal B}\gets1$
\If{$\operatorname{RMS}_{\mathcal B}(\Delta)>0$}
    \State $\widetilde d_{\mathcal B}\gets\operatorname{RMS}_{\mathcal B}(\Delta)/\operatorname{RMS}_{\mathcal B}(A^{S,\mathrm{ref}})$
\EndIf
\State $\widetilde A_t^{S,(i)}\gets\Delta_t^{(i)}/\widetilde d_{\mathcal B},\qquad \widetilde A_t^{(i)}\gets A^{E,(i)}+\beta\widetilde A_t^{S,(i)}$ for all visits
\State Assign each generated token the combined advantage of its step $\widetilde A_k$ and hold all advantages fixed

\For{each PPO minibatch $\mathcal M$ from $\mathcal B$}
    \State Apply normalized actor-loss weights $w_k^{\mathcal M}$, with $\sum_{k\in\mathcal M}w_k^{\mathcal M}=1$
    \State $\rho_k\gets\pi_\theta(a_k\mid h_k)/\pi_{\mathrm{old}}(a_k\mid h_k),\qquad \bar\rho_k\gets\operatorname{clip}(\rho_k,1-\epsilon,1+\epsilon)$ for all $k\in\mathcal M$
    \State $\mathcal J_{\mathcal M}(\theta)\gets\displaystyle\sum_{k\in\mathcal M}w_k^{\mathcal M}\left[\min(\rho_k\widetilde A_k,\bar\rho_k\widetilde A_k)-\lambda_{\mathrm{KL}}\mathbb D_{\mathrm{KL}}\!\left(\pi_\theta(\cdot\mid h_k)\,\middle\|\,\pi_{\mathrm{ref}}(\cdot\mid h_k)\right)\right]$
    \State Update $\theta$ with the configured optimizer to maximize $\mathcal J_{\mathcal M}(\theta)$
\EndFor
\State \Return $\pi_\theta$
\end{algorithmic}
\end{algorithm*}

\section{Diagnostic Analysis Details}
\label{app:diagnostics}
This section describes the analyses of relative-value calibration, continuation reuse, and computational cost for ConCal. All analyses reuse existing rollout data.

\paragraph{Relative-value evaluation.}
For the relative-value diagnostics in \figurename~\ref{fig:relative_calibration}, we analyze 30 frozen rollout batches per benchmark, collected at updates 5, 10, $\ldots$, 150. Within each task, we split the eight trajectories into two sets of four according to trajectory identifiers, independently of outcomes. Each estimator operates on one set, with sharing pools reconstructed within that set. Discounted returns from the other set provide the held-out reference. We then swap the two sets and repeat the evaluation. Across both split directions, we retain 592 comparison groups and 405 eligible action pairs for ALFWorld, and 334 groups and 137 pairs for WebShop.

Comparison groups share the same task, observed state, and remaining interaction budget. We retain groups containing at least two executed commands observed in both sets. For each command, we first average values within each trajectory. We then average the trajectory-level values with equal weights. Estimated and reference command values are centered separately within each group. Let $\mathbf z_g^m$ and $\mathbf z_g^{\mathrm{ref}}$ denote the centered vectors for estimator $m$ and the reference. We compute
\begin{equation}
    \operatorname{MSE}(m)
    =
    \frac{1}{|\mathcal G|}
    \sum_{g\in\mathcal G}
    \frac{
        \|\mathbf z_g^m-\mathbf z_g^{\mathrm{ref}}\|_2^2
    }{|\mathcal A_g|},
    \label{eq:diagnostic_centered_mse}
\end{equation}
where $\mathcal G$ contains all eligible comparison groups from both split directions across all batches, and $\mathcal A_g$ contains the commands observed in both sets for group $g$.
Ordering statistics include all unordered command pairs with an absolute reference gap of at least $10^{-3}$. Estimated gaps below $10^{-3}$ in absolute value are classified as \textit{Tie}. The remaining pairs are classified as \textit{Agreement} or \textit{Disagreement} according to whether their estimated direction matches the reference. Percentages are computed over all eligible pairs.

\paragraph{Gap-matched control.}
Gap-matched rescales the centered Own-MC vector within each comparison group:
\begin{equation}
    \mathbf z_g^{\mathrm{GM}}
    =
    \frac{
        \|\mathbf z_g^{\mathrm{ConCal}}\|_2
    }{
        \|\mathbf z_g^{\mathrm{MC}}\|_2
    }
    \mathbf z_g^{\mathrm{MC}}.
    \label{eq:gap_matched_control}
\end{equation}
When $\|\mathbf z_g^{\mathrm{MC}}\|_2\leq10^{-12}$, the original centered vector is retained. The scaling factor depends only on the estimator outputs, without held-out returns. When scaling is applied, the resulting vector has the same norm as the centered ConCal vector. Under this scaling, a positive factor preserves the Own-MC ordering and a zero target norm produces ties.

\paragraph{Evidence-reuse coverage.}
Coverage is measured on the same 30 complete batches per benchmark. An action has \textit{direct coverage} when its recorded successor belongs to a sharing pool containing visits from at least two distinct trajectories and the remaining continuation budget is positive. \textit{Additional recursive coverage} includes actions without direct coverage whose estimates incorporate cross-trajectory evidence through recursive updates within their remaining budget. All remaining actions are \textit{uncovered}. Coverage percentages are computed over all action occurrences in the analyzed batches, with each occurrence counted once.

\paragraph{Runtime measurement.}
Timings for rollout generation, policy updates, old-policy and reference-policy log-probability computation, and reward computation are taken from the original training logs over updates 2--150. Matching and recursive calibration are measured separately by replaying the frozen batches on an H100 MIG instance with 40\,GB of memory. These computations retain their CPU implementation. Calibration timing includes transferring and applying the correction on the GPU. CUDA is synchronized at stage boundaries. Each batch receives two warmup repetitions and seven timed repetitions per method. Component times are taken from the repetition with the median total replay time and averaged across batches. The runtime figure gives the two benchmark means equal weight.

\begin{figure*}[t!]
    \centering
    \includegraphics[width=1\textwidth]{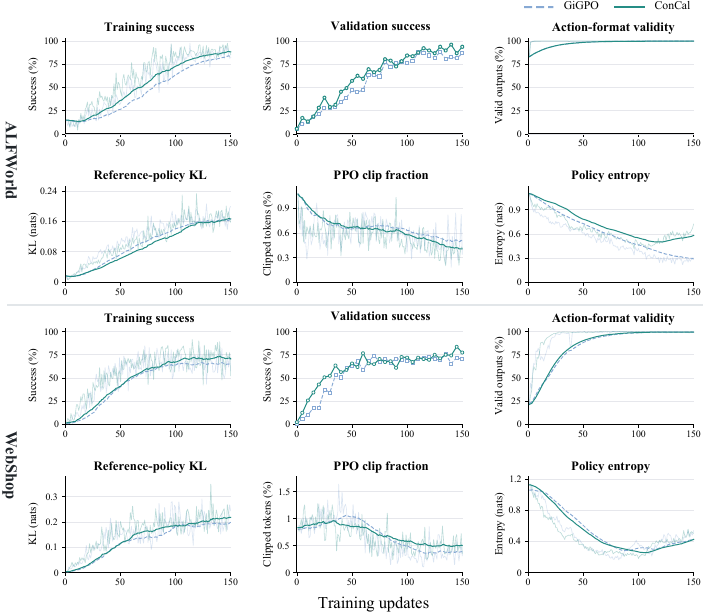}
    \caption{Training dynamics of ConCal and GiGPO with Qwen2.5-1.5B-Instruct. The top two rows show ALFWorld, and the bottom two rows show WebShop. Faint lines show raw training metrics, and bold lines show exponential moving averages with decay $0.95$. Validation success is shown at the recorded evaluation updates without smoothing.}
    \label{fig:additional_training_dynamics}
\end{figure*}

\section{Step-Advantage Normalization}
\label{app:step_normalization}
We compute step advantages through batch-wise normalization with a scale shared across all state groups in the complete rollout batch $\mathcal B$. Let $\Delta$ denote the group-centered calibrated action values. We compute reference advantages $A^{S,\mathrm{ref}}$ by applying the step-normalization rule in GiGPO to the same calibrated values. The rule performs group-wise standardization with the sample standard deviation plus $10^{-6}$ on ALFWorld and mean centering on WebShop.

Each generated token inherits its step-level value. With the normalized actor-loss weights $w_k$ from Eq.~\eqref{eq:concal_policy_objective}, the batch RMS is
\begin{equation}
    \operatorname{RMS}_{\mathcal B}(v)
    =
    \left(\sum_{k=1}^{L} w_k v_k^2\right)^{1/2}.
    \label{eq:batch_rms}
\end{equation}
When the centered-value RMS is nonzero, the shared normalization scale is
\begin{equation}
    \widetilde d_{\mathcal B}
    =
    \frac{
    \operatorname{RMS}_{\mathcal B}(\Delta)
    }{
    \operatorname{RMS}_{\mathcal B}(A^{S,\mathrm{ref}})
    }.
    \label{eq:batch_normalization_scale}
\end{equation}
On WebShop, $A^{S,\mathrm{ref}}=\Delta$ gives $\widetilde d_{\mathcal B}=1$. The scale is computed once over all tasks in the update and held fixed during policy optimization. If the centered-value RMS is zero, step advantages are set to zero. Episode-level advantages remain unchanged.


\section{Additional Training Dynamics}
\label{app:training_dynamics}
\figurename~\ref{fig:additional_training_dynamics} compares six learning and optimization metrics for ConCal and GiGPO from the same runs as the main-text learning curves. The metrics are training and validation success, action-format validity, reference-policy KL, PPO clip fraction, and policy entropy. Action-format validity measures compliance with the required response format, and the PPO clip fraction records how often the clipped surrogate determines the loss.

On ALFWorld, ConCal achieves higher training and validation success through much of training. On WebShop, the training-success advantage becomes clearer during later updates, with higher average training and validation success over the final 50 updates. Both methods reach nearly 100\% action-format validity on both benchmarks, while differences in task success persist.

The accompanying optimization dynamics vary across benchmarks. On ALFWorld, ConCal maintains higher policy entropy later in training, while the two methods reach similar reference-policy KL near the end. On WebShop, the higher late-stage success rates are accompanied by higher KL and clipping fractions. Both methods exhibit a similar decrease followed by a partial recovery in policy entropy on WebShop, and their clipping fractions decline during later training on both benchmarks.

\section{Discussion with Related Methods}
\label{app:method_discussion}

\subsection{GraphGPO}
\label{app:discussion_graphgpo}
GraphGPO~\citep{cheng2026graphgpo} constructs step rewards from shortest-path distances to successful terminal states. ConCal focuses on calibrating the action-value differences used for local credit. It recursively combines shared continuation evidence with each visit's own transition target, then evaluates actions using their recorded rewards and actual successors. Its credit therefore reflects estimated discounted returns, while GraphGPO's credit reflects distance to success on the merged graph. For actions from the same state with equal transition costs and equally distant successors, GraphGPO assigns identical distance-based step rewards. ConCal can still distinguish their action values through differences in recorded rewards and sampled continuation evidence, with partial sharing retaining each visit's contribution.

\subsection{SALT}
\label{app:discussion_salt}
SALT~\citep{li-etal-2026-salt} averages trajectory-level advantages across matched transitions to assign step-level credit. ConCal instead recursively calibrates continuation values by partially pooling targets $r+\gamma\widehat V$ across visits matched by their incoming transitions, retaining each visit's own transition contribution. It constructs action values from recorded rewards and calibrated continuation estimates at their actual successors, then derives local advantages through state-group centering. Recursive propagation also reaches earlier actions whose successor visits have no direct cross-trajectory match. SALT focuses on refining trajectory-level advantages into step-level credit, whereas our study centers on continuation-value estimation before local credit is formed. We provide an in-depth empirical analysis of how calibration changes preference strength and action ordering, and how normalization preserves or suppresses the resulting value gaps in local credit.

\subsection{GRAFT}
\label{app:discussion_graft}
Concurrent work GRAFT~\citep{yao2026graft} explicitly constructs a trajectory graph and estimates shared node values through empirical Bellman iteration. It derives step advantages from node-value differences and further refines them with Graph GAE. ConCal instead partially shares continuation evidence across visits matched by incoming transitions while retaining a separate estimate for each visit (Equation~\ref{eq:visit_difference}). Its recursive updates operate directly on recorded visits without explicitly constructing a transition graph. Action values combine recorded rewards with calibrated continuations at actual successors, with the state-group mean providing the local baseline. GRAFT focuses on graph-based state-value recovery and step-advantage construction, whereas our study centers on partial continuation calibration and its effects on relative action values. Using held-out returns, our in-depth empirical analysis distinguishes preference-strength calibration from action-order changes: Gap-matched reproduces most of ConCal's centered-MSE reduction relative to Own-MC through magnitude adjustment, while ConCal also improves ordering agreement.


\section{Prompt Templates}
\label{app:prompts}
We construct training and evaluation prompts from the environment templates provided by verl-agent~\citep{feng2025gigpo}. Each prompt contains the task, current observation, available actions, and up to two recent observation--action pairs. At each interaction step, we fill the placeholders in curly braces with the corresponding values. The prompts request reasoning within \texttt{<think>} tags and a single action within \texttt{<action>} tags.

\figurename{}s~\ref{fig:alfworld_prompt} and~\ref{fig:webshop_prompt} show the templates with interaction history. At the initial step, we select the corresponding template without interaction history. \figurename{}s~\ref{fig:alfworld_prompt_example} and~\ref{fig:webshop_prompt_example} show example user prompts from validation episodes on ALFWorld and WebShop, respectively.


\begin{figure*}[t]
\centering
\begin{lstlisting}[style=concalprompt]
You are an expert agent operating in the ALFRED Embodied Environment. Your task is to: {task_description}
Prior to this step, you have already taken {step_count} step(s). Below are the most recent {history_length} observations and the corresponding actions you took: {action_history}
You are now at step {current_step} and your current observation is: {current_observation}
Your admissible actions of the current situation are: [{admissible_actions}].

Now it's your turn to take an action.
You should first reason step-by-step about the current situation. This reasoning process MUST be enclosed within <think> </think> tags.
Once you've finished your reasoning, you should choose an admissible action for current step and present it within <action> </action> tags.
\end{lstlisting}
\caption{ALFWorld prompt template with interaction history. At the initial step, the task is included in the initial observation, and the history and step-index fields are omitted.}
\label{fig:alfworld_prompt}
\end{figure*}

\begin{figure*}[t]
\centering
\begin{lstlisting}[style=concalprompt]
You are an expert autonomous agent operating in the WebShop e‑commerce environment.
Your task is to: {task_description}.
Prior to this step, you have already taken {step_count} step(s). Below are the most recent {history_length} observations and the corresponding actions you took: {action_history}
You are now at step {current_step} and your current observation is: {current_observation}.
Your admissible actions of the current situation are:
[
{available_actions}
].

Now it's your turn to take one action for the current step.
You should first reason step-by-step about the current situation, then think carefully which admissible action best advances the shopping goal. This reasoning process MUST be enclosed within <think> </think> tags.
Once you've finished your reasoning, you should choose an admissible action for current step and present it within <action> </action> tags.
\end{lstlisting}
\caption{WebShop prompt template with interaction history. A template without history is selected at the initial step and when the formatted prompt exceeds 13,000 characters.}
\label{fig:webshop_prompt}
\end{figure*}

\begin{figure*}[t]
\centering
\begin{lstlisting}[style=concalprompt]
You are an expert agent operating in the ALFRED Embodied Environment. Your task is to: look at cd under the desklamp.
Prior to this step, you have already taken 3 step(s). Below are the most recent 2 observations and the corresponding actions you took: [Observation 2: 'You arrive at desk 1. On the desk 1, you see a cd 1, a cellphone 1, a creditcard 2, and a creditcard 1.', Action 2: 'take cd 1 from desk 1']
[Observation 3: 'You pick up the cd 1 from the desk 1.', Action 3: 'go to desk 2']
You are now at step 4 and your current observation is: You arrive at desk 2. On the desk 2, you see a book 1, a pen 2, a pen 1, and a pencil 2.
Your admissible actions of the current situation are: ['examine cd 1'
 'examine desk 2'
 'go to bed 1'
 'go to desk 1'
 'go to garbagecan 1'
 'go to shelf 1'
 'go to shelf 2'
 'go to shelf 3'
 'go to shelf 4'
 'go to shelf 5'
 'inventory'
 'look'
 'move cd 1 to desk 2'].

Now it's your turn to take an action.
You should first reason step-by-step about the current situation. This reasoning process MUST be enclosed within <think> </think> tags.
Once you've finished your reasoning, you should choose an admissible action for current step and present it within <action> </action> tags.
\end{lstlisting}
\caption{An example ALFWorld user prompt from a validation episode, showing the task, the two most recent interactions, the current observation, and available actions.}
\label{fig:alfworld_prompt_example}
\end{figure*}

\begin{figure*}[t]
\centering
\begin{lstlisting}[style=concalprompt,basicstyle=\footnotesize\ttfamily]
You are an expert autonomous agent operating in the WebShop e‑commerce environment.
Your task is to: Find me eco friendly, heavy duty, assembly required, easy clean file cabinets with size: 35.4"w x 15.7"d x 29.3"h, and price lower than 200.00 dollars.
Prior to this step, you have already taken 8 step(s). Below are the most recent 2 observations and the corresponding actions you took: [Observation 7: '[button] Back to Search [button_]
[button] < Prev [button_]
size
  [button] 23.6"w x 15.7"d x 29.3"h [button_]
  [button] 35.4"w x 15.7"d x 29.3"h [button_]
DEVAISE 2-Drawer Wood Lateral File Cabinet with Lock for Office Home, Black
Price: $169.99
Rating: N.A.
[button] Description [button_]
[button] Features [button_]
[button] Reviews [button_]
[button] Buy Now [button_]
', Action 7: 'click[35.4"w x 15.7"d x 29.3"h]']
[Observation 8: '[button] Back to Search [button_]
[button] < Prev [button_]
size
  [button] 23.6"w x 15.7"d x 29.3"h [button_]
  [button] 35.4"w x 15.7"d x 29.3"h [button_]
DEVAISE 2-Drawer Wood Lateral File Cabinet with Lock for Office Home, Black
Price: $169.99
Rating: N.A.
[button] Description [button_]
[button] Features [button_]
[button] Reviews [button_]
[button] Buy Now [button_]
', Action 8: 'click[35.4"w x 15.7"d x 29.3"h]']
You are now at step 9 and your current observation is: [button] Back to Search [button_]
[button] < Prev [button_]
size
  [button] 23.6"w x 15.7"d x 29.3"h [button_]
  [button] 35.4"w x 15.7"d x 29.3"h [button_]
DEVAISE 2-Drawer Wood Lateral File Cabinet with Lock for Office Home, Black
Price: $169.99
Rating: N.A.
[button] Description [button_]
[button] Features [button_]
[button] Reviews [button_]
[button] Buy Now [button_]
.
Your admissible actions of the current situation are:
[
'click[back to search]',
'click[< prev]',
'click[description]',
'click[features]',
'click[reviews]',
'click[buy now]',
'click[23.6"w x 15.7"d x 29.3"h]',
'click[35.4"w x 15.7"d x 29.3"h]',
].

Now it's your turn to take one action for the current step.
You should first reason step-by-step about the current situation, then think carefully which admissible action best advances the shopping goal. This reasoning process MUST be enclosed within <think> </think> tags.
Once you've finished your reasoning, you should choose an admissible action for current step and present it within <action> </action> tags.
\end{lstlisting}
\caption{An example WebShop user prompt from a validation episode, showing the shopping goal, the two most recent interactions, the current product page, and available actions.}
\label{fig:webshop_prompt_example}
\end{figure*}
